# Supplementary material for: Stereo Video Reconstruction Without Explicit Depth Maps for Endoscopic Surgery
Source: arXiv:2109.08227 source file (2021-09-16)
Supplement: Supplementary file 1 [file 7_supp_qual_examples.tex]

% \begin{figure}[p]
% \floatconts
%     {fig:animals}
%     {\caption{Generated images from the top eight models as ranked by the image-based reader study. Models are ranked from best \protect\subfigref{fig:111} to worst \protect\subfigref{fig:888}. Refer to \tableref{tab:models} for model descriptions and model performance.}}
%     {
%     \subfigure[][]{\label{fig:111}
%         \includegraphics[width=0.4\textwidth]{figs/qual_ranking/u22_pred_7.jpg}}
%     \qquad
%     \subfigure[][]{\label{fig:222}
%         \includegraphics[width=0.4\textwidth]{figs/qual_ranking/u3_pred_7.jpg}}

%     \subfigure[][]{\label{fig:333}
%         \includegraphics[width=0.4\textwidth]{figs/qual_ranking/u18_pred_7.jpg}}
%     \qquad
%     \subfigure[][]{\label{fig:444}
%         \includegraphics[width=0.4\textwidth]{figs/qual_ranking/s3_pred_7.jpg}}

%     \subfigure[][]{\label{fig:555}
%         \includegraphics[width=0.4\textwidth]{figs/qual_ranking/u13_pred_7.jpg}}
%     \qquad
%     \subfigure[][]{\label{fig:666}
%         \includegraphics[width=0.4\textwidth]{figs/qual_ranking/s8_pred_7.jpg}}

%     \subfigure[][]{\label{fig:777}
%         \includegraphics[width=0.4\textwidth]{figs/qual_ranking/s1_pred_7.jpg}}
%     \qquad
%     \subfigure[][]{\label{fig:888}
%         \includegraphics[width=0.4\textwidth]{figs/qual_ranking/u19_pred_7.jpg}}
%     }
% \end{figure}


% \begin{figure}[htbp]
%     \graphicspath{{figs/frame10_right_side/}}
%     \centering
%     \begin{subfigure}[b]{.18\textwidth}
%         \centering
%         \includegraphics[width=\textwidth]{target_10.jpg}
%         \caption{target}
%     \end{subfigure}
%     \begin{subfigure}[b]{.18\textwidth}
%         \centering
%         \includegraphics[width=\textwidth]{u22.jpg}
%         \caption{u22}
%     \end{subfigure}
%     \begin{subfigure}[b]{.18\textwidth}
%         \centering
%         \includegraphics[width=\textwidth]{u3.jpg}
%         \caption{u3}
%     \end{subfigure}
%     \begin{subfigure}[b]{.18\textwidth}
%         \centering
%         \includegraphics[width=\textwidth]{u18.jpg}
%         \caption{u18}
%     \end{subfigure}
%     \begin{subfigure}[b]{.18\textwidth}
%         \centering
%         \includegraphics[width=\textwidth]{s3.jpg}
%         \caption{s3}
%     \end{subfigure}
    
%     \begin{subfigure}[b]{.18\textwidth}
%         \centering
%         \includegraphics[width=\textwidth]{white-block.jpeg}
%     \end{subfigure}
%     \begin{subfigure}[b]{.18\textwidth}
%         \centering
%         \includegraphics[width=\textwidth]{u13.jpg}
%         \caption{u13}
%     \end{subfigure}
%     \begin{subfigure}[b]{.18\textwidth}
%         \centering
%         \includegraphics[width=\textwidth]{s8.jpg}
%         \caption{s8}
%     \end{subfigure}
%     \begin{subfigure}[b]{.18\textwidth}
%         \centering
%         \includegraphics[width=\textwidth]{s1.jpg}
%         \caption{s1}
%     \end{subfigure}
%     \begin{subfigure}[b]{.18\textwidth}
%         \centering
%         \includegraphics[width=\textwidth]{u19.jpg}
%         \caption{u19}
%     \end{subfigure}
% \caption{Cropped right most section of frame 10 - most uncertainty here}
% \label{fig:qual_rank_comparison2}
% \end{figure}
